# Supplementary material for: Improving Actor-Critic Reinforcement Learning via Hamiltonian Monte Carlo Method
Source: arXiv:2103.12020 source file (2022-01-02)
Supplement: Supplementary file 1 [file appendix_uai.tex]

\clearpage

\appendix

%\begin{table}[H]
%    \centering
%    \begin{tabular}{p{1.3in}<{\centering}|p{0.3in}<{\centering}|p{0.3in}<{\centering}|p{0.3in}<{\centering}|p{0.3in}<{\centering}|p{0.4in}<{\centering}}
%    \hline
%         & $K$ & $l$ & $h$ & $m$ & $\mathcal{B}$ size \\\hline
%    HalfCheetah-v2 & 3 & 1 & 32 & \multirow{8}*{256} & \multirow{8}*{$10^6$} \\
%    Hopper-v2 & 2 & 1 & 32 &  &  \\
%    Walker2d-v2 & 3 & 1 & 32 &  &  \\
%    Ant-v2 & 3 & 1 & 32 &  &  \\
%    Humanoid-v2 & 3 & 1 & 64 &  &  \\
%    Humanoid PyBullet & 3 & 1 & 64 & & \\
%    \makecell[c]{Humanoid Flagrun \\ PyBullet} & 3 & 1 & 32 & & \\
%    \makecell[c]{Humanoid Flagrun \\ Harder PyBullet} & 3 & 1 & 64 & & \\
%    \hline
%    \end{tabular}
%    \makeatletter\def\@captype{table}\makeatother\caption{Important Hyperparameters in SAC-HPO.}
%    \label{tab:mujoco_hyp}
%\end{table}

\section{Algorithm}
\label{sec:appendix_alg}
